# Supplementary material for: DualFed: Enjoying both Generalization and Personalization in Federated Learning via Hierachical Representations
Source: arXiv:2407.17754 source file (2025-02-05)
Supplement: Supplementary file 1 [file supplementary.pdf]

# Supplementary Materials - DualFed: Enjoying both Generalization and Personalization in Federated Learning via Hierachical Representations

## 1 Algorithm Details for DualFed

The training procedure for DualFed is presented in Algorithm 1. It mainly consists of the following steps within a single global round:

- The sever sends a global encoder and classifier to each client.
- Each client loads the parameters from the received global encoder and classifier into its local ones, then iteratively updates the main branch (including the global encoder, the personalized projector, and the personalized classifier) and the global classifier using its local data.
- Once local updating is completed, each client uploads its latest global encoder and classifier to the server.
- The sever aggregates these uploaded global encoder and classifier to generate the new ones.

The above steps are repeated until the model converges.

**Algorithm 1** DualFed

**Notations:** $T$: global updating rounds, $E$: local updating epochs, $B$: local minibatch size, $\eta$: learning rate, $\lambda$: loss-balanced hyperparameters, $\theta_m^{f,s,t}$: parameters of global encoder, $\theta_m^{h,s,t}$: parameters of global classifier, $\theta_m^{g,p,t}$: parameters of personalized projection network, $\theta_m^{h,p,t}$: parameters of personalized classifier, $\Theta_m^t := \{\theta_m^{f,s,t}, \theta_m^{h,s,t}, \theta_m^{g,p,t}, \theta_m^{h,p,t}\}$: parameters of local model, $\overline{\Theta}_m^t := \{\theta_m^{f,s,t}, \theta_m^{g,p,t}, \theta_m^{h,p,t}\}$: parameters of main branch, $\tilde{\theta}^{f,s,t}$: aggregated parameters of global encoder, $\tilde{\theta}^{h,s,t}$: aggregated paramters of global classifier.

**Sever Executes:**

*# model initialization*
broadcast initialized model $\Theta^1$ to each client
**for** $t = 1, 2, 3, \ldots, T$ **do**
  *# performing local updating*
  **for** each client $m$ **in parallel do**
    $\theta_m^{f,s,t+1}, \theta_m^{h,s,t+1} \leftarrow \text{ClientUpdate}(m, t, \tilde{\theta}^{f,s,t}, \tilde{\theta}^{h,s,t})$
  **end for**
  *# aggregating global encoder and classifier*
  $\tilde{\theta}^{f,s,t+1} = \sum_{m=1}^{M} \frac{1}{M} \theta_m^{f,s,t+1}$, $\tilde{\theta}^{h,s,t+1} = \sum_{m=1}^{M} \frac{1}{M} \theta_m^{h,s,t+1}$
**end for**

**ClientUpdate**($m, t, \tilde{\theta}^{f,s,t}, \tilde{\theta}^{h,s,t}$)**:**

*# loading global encoder and classifier*
$\theta_m^{f,s,t} \leftarrow \tilde{\theta}^{f,s,t}$, $\theta_m^{h,s,t} \leftarrow \tilde{\theta}^{h,s,t}$
*# updating main branch*
$\mathcal{B} \leftarrow$ (split local dataset into batches of size B)
**for** $i = 1, 2, 3, \ldots, E$ **do**
  **for** batch $(\boldsymbol{x}_b, \boldsymbol{y}_b) \in \mathcal{B}$ **do**
    $\boldsymbol{z} = f(\boldsymbol{x}_b; \theta_m^{f,s,t}), \boldsymbol{u} = f(\boldsymbol{z}; \theta_m^{g,p,t}), \hat{\boldsymbol{y}}^p = f(\boldsymbol{u}; \theta_m^{h,p,t})$
    $\overline{\Theta}_m^t \leftarrow \overline{\Theta}_m^t - \eta \nabla_{\overline{\Theta}_m^t} \mathcal{L}_{pcls}(\hat{\boldsymbol{y}}^p, \boldsymbol{y}_b) + \lambda \mathcal{L}_{con}(\boldsymbol{u})$
  **end for**
**end for**
*# updating global classifier*
$\mathcal{B} \leftarrow$ (split local dataset into batches of size B)
**for** $i = 1, 2, 3, \ldots, E$ **do**
  **for** batch $(\boldsymbol{x}_b, \boldsymbol{y}_b) \in \mathcal{B}$ **do**
    $\boldsymbol{z} = f(\boldsymbol{x}_b; \theta_m^{f,s,t}), \hat{\boldsymbol{y}}^s = f(\boldsymbol{z}; \theta_m^{h,s,t})$
    $\theta_m^{h,s,t} \leftarrow \theta_m^{h,s,t} - \eta \nabla_{\theta_m^{h,s,t}} \mathcal{L}_{scls}(\hat{\boldsymbol{y}}^s, \boldsymbol{y}_b)$
  **end for**
**end for**
$\theta_m^{g,p,t+1} \leftarrow \theta_m^{g,p,t}$, $\theta_m^{h,p,t+1} \leftarrow \theta_m^{h,p,t}$
return $\theta_m^{f,s,t+1}, \theta_m^{h,s,t+1}$ to server

## 2 Dataset Description

Our experiments are conducted on three datasets: PACS [8], DomainNet [15], and Office-Home [17]. The PACS dataset includes 4 distinct domains: Photo (P), Art (A), Cartoon (C), and Sketch (S), each containing images from 7 common classes. The DomainNet dataset encompasses 6 distinct domains: Clipart (C), Infograph (I), Painting (P), Quickdraw (Q), Real (R), and Sketch (S). Initially, each domain in DomainNet dataset comprises 345 classes. Following previous studies [10, 18], we narrow these domains down to 10 commonly-used classes to create our experimental dataset. The Office-Home dataset contains images from 4 distinct domains: Art (A), Clipart (C), Product (P), and Real-World (R), each containing 65 classes. We retain all classes in Office-Home to conduct a comprehensive evaluation of DualFed on a larger-scale scenario. Figure 1 presents some example images in these three datasets. For each domain, we show the images from 5 representing classes. It can be observed that significant variations exist among different domains, suggesting that personalized representations can vary considerably across these domains. Therefore, it is crucial to explore both generalized representations shared across these domains and personalized representations specific to each domain to enhance collaboration in federated learning (FL) with heterogenous data.

For these three datasets, we select the images from a single domain to form the dataset of an individual client. Consequently, there are 4 clients for PACS, 6 clients for DomainNet, and 4 clients for Office-Home, respectively. In both PACS and DomainNet datasets, we chose a subset of 500 training images per client from the same domain to comprise the training dataset. For Office-Home daatset, we consider a more extensive experimental scenario with more samples. We set the number of training samples to 2,000 for the Clipart, Product, and Real-World domains. In the case of the Art domain, the number is limited to 1,942, matching the total number of samples available in this domain. All the images from the test dataset are reserved for evaluation for these datasets. In line with the experimental settings of previous studies, the images are resized to $256 \times 256$ for DomainNet, $227 \times 227$ for PACS, and $224 \times 224$

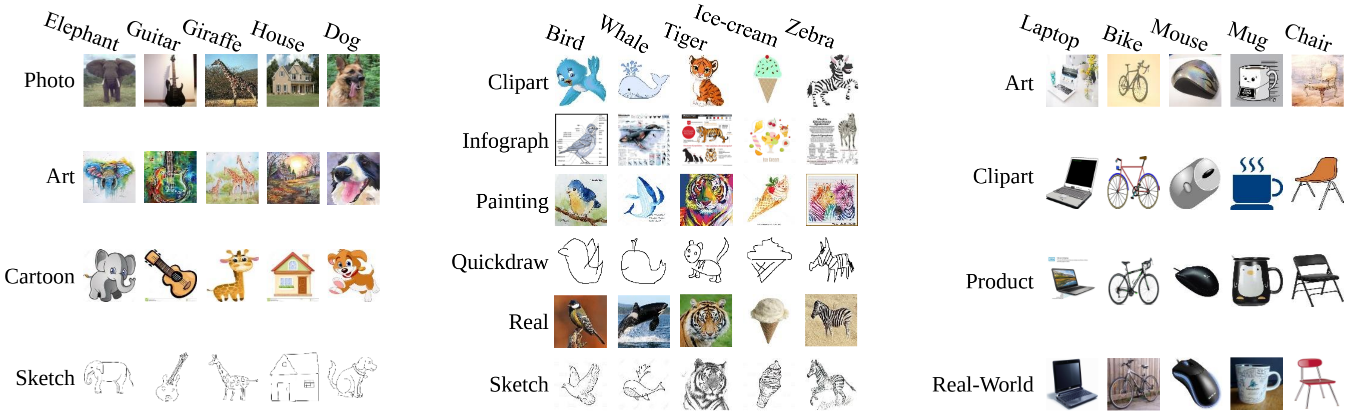


(a) PACS (b) DomainNet (c) Office-Home

**Figure 1: Visualization of example images in the adopted dataset, (a) PACS, (b)DomainNet, (c)Office-Home. We present images from 5 classes for each domain in these datasets.**

for Office-Home, respectively, before feeding into the model. Additionally, we apply random flipping and rotational augmentations to these images during the training.

## 3 Implementation Details of Experiments

In our experiments, we compare DualFed with multiple benchmark FL methods, including FedAvg[13], FedProx[9], FedPer[1], FedRep[3], LG-FedAvg[12], FedBN[10], FedProto[16], SphereFed[4], Fed-RoD[2], FedETF[11]. Additionally, the SingleSet method, where separate models are trained and tested for each client using only their private data, is also used for comparison in our experiments. We reproduce these FL methods based on the discussions in their original paper and the official code [1,2,3,4,5], when available.

We modify the ResNet18 model, originally pretrained on the ImageNet dataset, by removing its final fully connected (FC) layer, thereby transforming it into an encoder [5]. This encoder is followed by a projector network, which consists of an FC network with the architecture: [Linear(512, 256) - ReLU - BN - Linear(256, 512) - BN]. To ensure uniform model capacity, all compared methods employ this Encoder-Projector architecture for representation extraction, with only specific alterations made to the classifiers in some approaches. Specifically, SphereFed initializes its classifier orthogonally and maintains it unchanged throughout the training process. In FedETF, the classifier is initialized as an ETF (Equiangular Tight Frame) architecture and kept fixed during the training. FedRoD employs both global and personalized classifiers simultaneously during training. All classifiers utilized in our experiments consist of an FC layer, with 512 input neurons and a number of output neurons that matches the class count.

We conduct all experiments on a Nvidia V100 four-card cluster, utilizing the PyTorch [14] framework. The model is optimized by stochastic gradient descent (SGD) with momentum. The learning rate is consistently set at 0.01, with a momentum of 0.5, applicable to all methods except SphereFed. Due to the differing loss value magnitudes in SphereFed compared to other methods [4], we carefully adjust its learning rates for each dataset. Consequently, we set the learning rate to 1.0 for Office-Home and to 0.1 for both DomainNet and PACS. During local updates, a batch size of 256 is consistent across all methods. The epoch of local updating is set to 1 for all methods except FedRep. For FedRep, it has a total of 5 local epochs, with the initial 4 epochs focusing on classifier optimization and the last epoch on encoder and projector optimization. The total count of global rounds is set to 300 for all methods.

In our experiments with FedProx, we set the hyperparameter $\mu$—responsible for balancing the loss terms—to 0.01 for all datasets. After extensive searching, we set the hyperparameter for aligning global and local prototypes in FedProto to 1.0 across all datasets. For DualFed, the temperature for representation contrastive learning is set to 0.2 for PACS, and 0.05 for DomainNet and OfficeHome. The $\lambda$ used to balance the cross entropy loss and contrastive loss is set to 40, 10 and 2 for PACS, DomainNet, and Office-Home, respectively.

To mitigate cross-domain interference and potential privacy issues related to batch normalization (BN) layers, we localize the *running-mean* and *running-var* components within these layers for all methods.

The stage of model evaluation, a critical factor for comparison, is determined based on the settings described in the original papers of the compared FL methods. For FedETF, the model is evaluated after local finetuning on each client. According to its official source code [5], the global model in FedETF is finetuned for 1 round firstly, then the ETF classifier and projection network are alternately finetuned for 20 rounds. In each of alternative finetuned rounds, both the ETF classifier and projection layer are finetuned for 3 rounds. Apart from FedETF, all other methods undergo evaluation post model aggregation. It should be noted that although SphereFed proposes to conduct model evaluation after the fast federated calibration (FFC), we find this operation is harmful to the model in our settings and report the accuracy after the model aggregation.

[1]https://github.com/litian96/FedProx
[2]https://github.com/med-air/FedBN
[3]https://github.com/yuetan031/FedProto
[4]https://github.com/hongyouc/Fed-RoD
[5]https://github.com/ZexiLee/ICCV-2023-FedETF

**Table 1: Experiments with Different Projector Architecture.**

| $D$ | $H$ | BN | Detailed Architecture | PACS | DomainNet | Office-Home |
|---|---|---|---|---|---|---|
| 1 | 256 | ✓ | [Linear(512, 512) - BN] | 94.72±0.18 | 86.16±0.09 | 79.96±0.24 |
| 2 | 256 | ✓ | [Linear(512, 256) - ReLU - BN - Linear(256, 512) - BN] | 95.01±0.31 | 86.14±0.12 | 79.74±0.37 |
| 3 | 256 | ✓ | [Linear(512, 256) - ReLU - BN -Linear(256, 256) - ReLU - BN - Linear(256, 512) - BN] | 94.97±0.18 | 85.91±0.26 | 79.31±0.36 |
| 2 | 64 | ✓ | [Linear(512, 64) - ReLU - BN - Linear(64, 512) - BN] | 95.35±0.19 | 86.06±0.32 | 79.43±0.24 |
| 2 | 128 | ✓ | [Linear(512, 128) - ReLU - BN - Linear(128, 512) - BN] | 95.15±0.18 | 85.95±0.18 | 79.49±0.21 |
| 2 | 512 | ✓ | [Linear(512, 512) - ReLU - BN - Linear(512, 512) - BN] | 95.21±0.17 | 86.23±0.23 | 79.97±0.35 |
| 2 | 256 | ✗ | [Linear(512, 256) - ReLU - Linear(256, 512)] | 95.13±0.19 | 86.23±0.26 | 79.22±0.38 |

During the experiments, we choose the accuracy on the test dataset as the metric to quantifying the model performance. To ensure the reliability of our results, each experiment is repeated 5 times with different random seeds: $\{0, 1, 2, 3, 4\}$. We report the mean and standard deviation of the highest test accuracy achieved during FL training for all methods.

# 4 Additional Analysis of DualFed

## 4.1 Effect of Projection Network Architecture

We investigate the impact of the architecture of the projection network in three key aspects: the depth of projection network ($D$), the dimension of hidden layers ($H$), the impact of BN layers. In the experiments, we set $D$ to $\{1, 2, 3\}$ and $H$ to $\{64, 128, 256, 512\}$, respectively. The detailed architecture of projectoion network and the corresponding results are shown in Table 1. From Table 1, we can derive the following conclusions. While increasing $D$ can lead to more generalized pre-projection representations, it simultaneously reduces their discriminative power. Therefore, it is advisable to select an optimal $D$ that maintains a balance in the discriminative and generalized ability of the pre-projection representations. Increasing $H$ can enhance the model performance in most times, as it enables the task-relevant information within the post-projection representations to be effectively passed to the pre-projection representations. The importance of BN layers becomes more pronounced as the scale of the dataset increases.

## 4.2 Quantitative evaluation of representations

We employ two metrics to quantitatively evaluate the evolution of generalized and personalized representations during training. To quantify the generalization of representations, we adopt the *linear centered kernel alignment (CKA)* [7] to measure the similarity of representations across clients. This metric is resistant to rotation and isotropic scaling in the representation space, allowing us to effectively measure the similarity of representations across clients.

With a little abuse of notations, we define $Z_i \in \mathbb{R}^{n_i \times k}$ and $Z_j \in \mathbb{R}^{n_j \times k}$ as two stacked representations (can be pre-projection representations or post-projector representations) on client $i$ and $j$ respectively. Here, $n_i$ and $n_j$ represent the number of samples on client $i$ and client $j$ respectively, and $k$ the dimension of representations. The original linear CKA is used to calculate the similarity between representations generated by the same dataset but at the different stages in the model. However, in this paper, we use it to measure the similarity of the representation of different clients in the same dimension, which is calculated as follows:

$$CKA_{linear}(Z_i, Z_j) = \frac{\text{vec}(\text{cov}(Z_i^T)) \cdot \text{vec}(\text{cov}(Z_j^T))}{||\text{cov}(Z_i^T)||_F ||\text{cov}(Z_j^T)||_F}, \quad (1)$$

where $\text{cov}(\cdot)$ denotes the covariance matrices, $||\cdot||_F$ denotes the Frobenius norm. Higher linear CKA values indicate greater similarity between two representations of different clients in the same dimension.

Additionally, we adopt the within-class variance in [6], to measure the class-wise *separation* of representation on local clients. This metric is determined by the ratio of the average within-class cosine distance, denoted by $\bar{d}within$, to the overall average cosine distance, denoted by $\bar{d}total$. The one minus operation is performed to this ratio to get a closed-form index of class separation that is between 0 and 1, as follows:

$$R^2 = 1 - \frac{\bar{d}_{within}}{\bar{d}_{total}}. \quad (2)$$

Given an arbitrary client $m$, $\bar{d}_{within}$ and $\bar{d}_{total}$ are calculated as follows:

$$\bar{d}_{within} = \sum_{c=1}^{C} \sum_{i=1}^{N_m^c} \sum_{j=1}^{N_m^c} \frac{1 - z_m^{c,i} \odot z_m^{c,j}}{C(N_m^c)^2}, \quad (3)$$

$$\bar{d}_{total} = \sum_{c=1}^{C} \sum_{k=1}^{C} \sum_{i=1}^{N_m^c} \sum_{j=1}^{N_m^k} \frac{1 - z_m^{c,i} \odot z_m^{k,j}}{C^2 N_m^c N_m^k}, \quad (4)$$

where $\odot$ is the cosine similarity, and $N_m^c$ indicates the number of samples belonging to class $C$ on client $m$.

Figure 2 presents the varying of $R^2$ during training. It can be seen that the personalized representations can achieve higher separation compared with the generalized representations. However, as shown in Figure 3, the similarity between clients of generalized representations is significant higher that that of the personalized representations. This demonstrates the DualFed can effectively decouple the optimization objectives of PFL (personalized federated learning) into two stages of the model representation extraction.

## 4.3 Comparison of Training Strategy

DualFed employs a stage-wise training strategy, ensuring that the pre-projection representation remain undisturbed by specific local

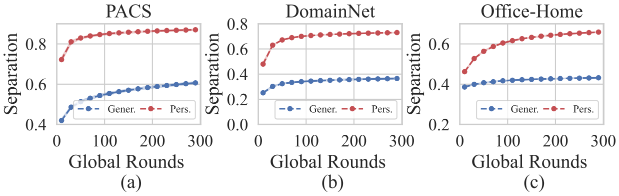


**Figure 2: Class-wise separation during training.**

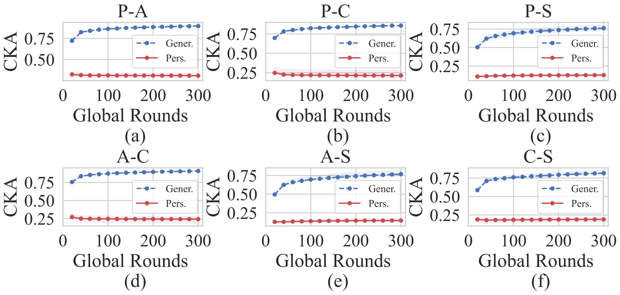


**Figure 3: Client-wise CKA similarity during training.**

tasks, thereby maintaining its generalization. Here, we compare this training strategy with the one that training all parameters simultaneously. Figure 4 presents the comparison of these two training strategies. As shown in Table 2, when $E$ is relatively small (i.e., $E = 1$), simultaneous training can, in fact, outperforms stage-wise training. However, as $E$ increases (i.e., $E = 20$), simultaneous training lead to a obvious performance drop in PACS and DomainNet. This trend can be attributed to the fact that an increased number of local epochs causes the pre-projection representations to align more closely with the local task, thereby reducing their generalization.

**Table 2: Experiments with Different Training Strategy.**

| $E$ | Strategy | PACS | DomainNet | Office-Home |
|---|---|---|---|---|
| 1 | Stage-wise | 95.01±0.31 | 86.14±0.12 | 79.74±0.37 |
| | Simu. | 95.15±0.16 | 86.68±0.20 | 80.57±0.09 |
| 20 | Stage-wise | 94.17±0.28 | 84.49±0.18 | 75.93±0.77 |
| | Simu. | 93.85±0.30 | 84.71±0.33 | 75.42±0.65 |

## 4.4 Effect of Position of Global Classifier

In DualFed, we employ a global classifier for generalized representations and a personalized classifier for personalized representations. Here we conduct experiments when placing the global classifier to the personalized representations. In these experiments, we maintain a shared encoder and investigated two configurations: sharing the projection network (DualFed-G) and personalizing it (DualFed-P). Figure 5 presents the differences of the above two configurations, along with the original DualFed. As indicated in Table 3, removing the global classifier to the same stage as the personalized classifier results in a significant performance decrease. This observation underscores the importance of the representations at different stages, as they provide complementary information (both generalized and personalized information) that can enhance the overall performance of the model.

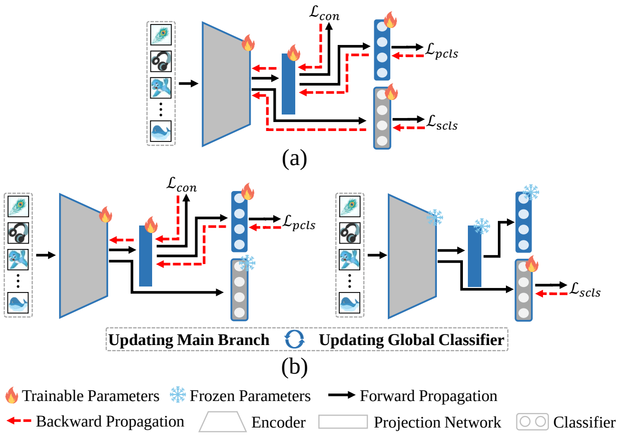


**Figure 4: Illustration of different training strategies, (a) Simultaneous training, (b) Stage-wise training.**

**Table 3: Experimental Results when Placing Global Classifier at Different Positions.**

| | PACS | DomainNet | Office-Home |
|---|---|---|---|
| DualFed | 95.01±0.31 | 86.14±0.12 | 79.74±0.37 |
| DualFed-P | 94.95±0.18 | 85.55±0.09 | 78.24±0.29 |
| DualFed-G | 94.84±0.12 | 84.90±0.42 | 78.08±0.17 |

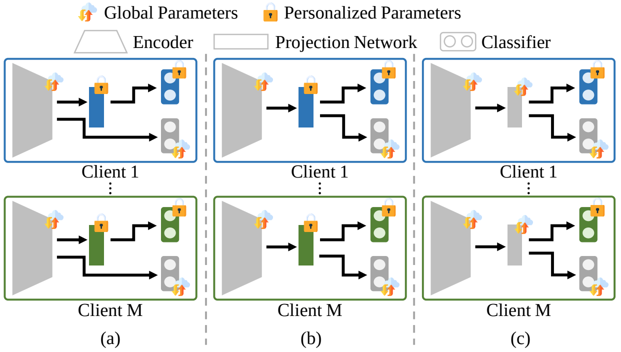


**Figure 5: Illustration of different positions of the global classifier, (a) DualFed, (b) DualFed-P, (c) DualFed-G.**

# References


[1] Manoj Ghuhan Arivazhagan, Vinay Aggarwal, Aaditya Kumar Singh, and Sunav Choudhary. 2019. Federated learning with personalization layers. *arXiv preprint arXiv:1912.00818* (2019).

[2] Hong-You Chen and Wei-Lun Chao. 2022. On Bridging Generic and Personalized Federated Learning for Image Classification. In *International Conference on Learning Representations*.

[3] Liam Collins, Hamed Hassani, Aryan Mokhtari, and Sanjay Shakkottai. 2021. Exploiting shared representations for personalized federated learning. In *International Conference on Machine Learning*. PMLR, 2089–2099.

[4] Xin Dong, Sai Qian Zhang, Ang Li, and HT Kung. 2022. Spherefed: Hyperspherical federated learning. In *European Conference on Computer Vision*. Springer, 165–184.

[5] Kaiming He, Xiangyu Zhang, Shaoqing Ren, and Jian Sun. 2016. Deep residual learning for image recognition. In *Proceedings of the IEEE conference on computer vision and pattern recognition*. 770–778.

[6] Simon Kornblith, Ting Chen, Honglak Lee, and Mohammad Norouzi. 2021. Why do better loss functions lead to less transferable features? *Advances in Neural Information Processing Systems* 34 (2021), 28648–28662.

[7] Simon Kornblith, Mohammad Norouzi, Honglak Lee, and Geoffrey Hinton. 2019. Similarity of neural network representations revisited. In *International conference on machine learning*. PMLR, 3519–3529.

[8] Da Li, Yongxin Yang, Yi-Zhe Song, and Timothy M Hospedales. 2017. Deeper, broader and artier domain generalization. In *Proceedings of the IEEE international conference on computer vision*. 5542–5550.

[9] Tian Li, Anit Kumar Sahu, Manzil Zaheer, Maziar Sanjabi, Ameet Talwalkar, and Virginia Smith. 2020. Federated optimization in heterogeneous networks. *Proceedings of Machine learning and systems* 2 (2020), 429–450.

[10] Xiaoxiao Li, Meirui JIANG, Xiaofei Zhang, Michael Kamp, and Qi Dou. 2021. FedBN: Federated Learning on Non-IID Features via Local Batch Normalization. In *International Conference on Learning Representations*.

[11] Zexi Li, Xinyi Shang, Rui He, Tao Lin, and Chao Wu. 2023. No Fear of Classifier Biases: Neural Collapse Inspired Federated Learning with Synthetic and Fixed Classifier. In *Proceedings of the IEEE/CVF International Conference on Computer Vision (ICCV)*. 5319–5329.

[12] Paul Pu Liang, Terrance Liu, Liu Ziyin, Nicholas B Allen, Randy P Auerbach, David Brent, Ruslan Salakhutdinov, and Louis-Philippe Morency. 2020. Think locally, act globally: Federated learning with local and global representations. *arXiv preprint arXiv:2001.01523* (2020).

[13] Brendan McMahan, Eider Moore, Daniel Ramage, Seth Hampson, and Blaise Aguera y Arcas. 2017. Communication-efficient learning of deep networks from decentralized data. In *Artificial intelligence and statistics*. PMLR, 1273–1282.

[14] Adam Paszke, Sam Gross, Francisco Massa, Adam Lerer, James Bradbury, Gregory Chanan, Trevor Killeen, Zeming Lin, Natalia Gimelshein, Luca Antiga, et al. 2019. Pytorch: An imperative style, high-performance deep learning library. *Advances in neural information processing systems* 32 (2019).

[15] Xingchao Peng, Qinxun Bai, Xide Xia, Zijun Huang, Kate Saenko, and Bo Wang. 2019. Moment matching for multi-source domain adaptation. In *Proceedings of the IEEE/CVF international conference on computer vision*. 1406–1415.

[16] Yue Tan, Guodong Long, Lu Liu, Tianyi Zhou, Qinghua Lu, Jing Jiang, and Chengqi Zhang. 2022. Fedproto: Federated prototype learning across heterogeneous clients. In *Proceedings of the AAAI Conference on Artificial Intelligence*, Vol. 36. 8432–8440.

[17] Hemanth Venkateswara, Jose Eusebio, Shayok Chakraborty, and Sethuraman Panchanathan. 2017. Deep hashing network for unsupervised domain adaptation. In *Proceedings of the IEEE conference on computer vision and pattern recognition*. 5018–5027.

[18] Fu-En Yang, Chien-Yi Wang, and Yu-Chiang Frank Wang. 2023. Efficient model personalization in federated learning via client-specific prompt generation. In *Proceedings of the IEEE/CVF International Conference on Computer Vision*. 19159–19168.
